# Supplementary material for: Spatial Information Bottleneck for Interpretable Visual Recognition
Source: arXiv:2511.09239 source file (2026-09-24)
Supplement: Supplementary file 1 [file supplementary.pdf]

# Supplementary Material for Spatial Information Bottleneck for Interpretable Visual Recognition

Paper ID: 11181

The implementation code for our method is available at the anonymous repository: https://anonymous.4open.science/r/S-IB-132E.

## 1. Implementation Details of Differentiable Mask Generator

In the main paper, we proved that the differentiable mask generation preserves sufficiency (Proposition 1). Here, we provide the concrete implementation of the mask generator $g : \mathbb{R}^{h\times w} \to [0,1]^{h\times w}$.

The key challenge is replacing non-differentiable operations (hard thresholding, exact quantile computation) with smooth, differentiable approximations. Our implementation consists of two main components: (1) differentiable quantile approximation via softmax weighting (Section 1.1), and (2) density-based mask generation with soft thresholding (Section 1.2).The complete procedure is summarized in Algorithm 1.

**Algorithm 1** Differentiable Mask Generation

**Require:** Relevance map $R \in \mathbb{R}^{h\times w}$
**Ensure:** Soft mask $M \in [0,1]^{h\times w}$
**Parameters:** $\tau = 0.1$, $\beta = 10$, $k = 31$

*// Normalization*
$R_{\text{gray}} \leftarrow |R|$
$r_{\min} \leftarrow \text{Quantile}_\tau(R_{\text{gray}}, 0.05)$
$r_{\max} \leftarrow \text{Quantile}_\tau(R_{\text{gray}}, 0.95)$
$R_{\text{norm}} \leftarrow (R_{\text{gray}} - r_{\min})/(r_{\max} - r_{\min} + 10^{-8})$

*// Adaptive soft thresholding*
$t_1 \leftarrow \text{Quantile}_\tau(R_{\text{norm}}, 0.8)$
$R_{\text{high}} \leftarrow \sigma(\beta \cdot (R_{\text{norm}} - t_1))$

*// Density-based refinement*
$D \leftarrow \text{AvgPool}_{k\times k}(R_{\text{high}})$
$t_2 \leftarrow \text{Quantile}_\tau(D, 0.8)$
$M \leftarrow \sigma(\beta \cdot (D - t_2))$

**return** $M$

### 1.1. Differentiable Quantile Approximation

Standard quantile computation involves sorting the input and selecting the element at a specific index, which is non-differentiable. We propose a smooth approximation using temperature-controlled softmax weighting.

#### 1.1.1. Formulation

Given an input tensor $\mathbf{x} \in \mathbb{R}^n$ and target quantile $q \in [0,1]$, the exact $q$-quantile selects the value at index $\lfloor q(n-1) \rfloor$ in the sorted sequence. We approximate this by:

$$\text{Quantile}_\tau(\mathbf{x}, q) = \sum_{i=0}^{n-1} x^{(i)}_{\text{sorted}} \cdot w_i \qquad (1)$$

where $x^{(i)}_{\text{sorted}}$ denotes the $i$-th element in the sorted sequence, and the weights are computed as:

$$w_i = \frac{\exp\left(-|i - q(n-1)|/\tau\right)}{\sum_{j=0}^{n-1} \exp\left(-|j - q(n-1)|/\tau\right)} \qquad (2)$$

Here, $\tau > 0$ is a temperature parameter. As $\tau \to 0$, the weights concentrate around the true quantile index, recovering exact quantile computation. In practice, we use $\tau = 0.1$ to balance approximation accuracy and gradient smoothness.

#### 1.1.2. Properties

This approximation has two key properties:

- **Differentiability**: Since PyTorch's sorting operation is differentiable and softmax is smooth, the entire computation graph supports backpropagation.
- **Approximation quality**: The softmax weights decay exponentially with distance from the target index, ensuring the weighted sum is dominated by nearby elements.

### 1.2. Density-Based Mask Generation

Given a relevance map $R \in \mathbb{R}^{h\times w}$, we generate the soft mask $M = g(R)$ through the following pipeline.

#### 1.2.1. Step 1: Robust Normalization

We first convert to grayscale and take absolute values:

$$R_{\text{gray}} = |R| \qquad (3)$$

Table 1. Quantitative comparison of post-hoc explanation methods on ResNet-18. Format: Baseline→Ours.

| Method | CUB-200 | | | Oxford-IIIT Pet | | | Stanford Dogs | | |
|---|---|---|---|---|---|---|---|---|---|
| | Pixel Acc | mIoU | mAP | Pixel Acc | mIoU | mAP | Pixel Acc | mIoU | mAP |
| Saliency | 78.35→78.46 | 39.38→39.40 | 40.69→42.42 | 59.12→59.13 | 29.72→29.78 | 69.56→69.57 | 27.09→27.17 | 13.59→13.71 | 87.83→87.89 |
| GuidedBackprop | 78.34→78.43 | 39.26→39.29 | 58.03→58.89 | 59.04→59.07 | 29.58→29.59 | 59.66→59.98 | 26.99→27.21 | 13.51→13.63 | 87.35→87.68 |
| IntegratedGradients | 78.37→78.41 | 39.37→39.40 | 46.97→48.61 | 59.09→59.12 | 29.67→29.69 | 65.54→65.58 | 27.05→27.32 | 13.56→13.59 | 87.12→87.27 |
| GradCAM | 79.09→79.55 | 58.24→58.79 | 62.83→63.90 | 73.94→74.23 | 55.60→56.10 | 76.76→76.87 | 57.66→57.89 | 40.28→40.43 | 91.69→91.95 |
| GradCAM++ | 77.30→77.98 | 57.81→58.55 | 69.54→70.34 | 74.98→75.26 | 57.10→57.32 | 78.10→79.24 | 59.91→60.03 | 42.34→42.45 | 91.90→92.34 |
| ScoreCAM | 78.26→78.93 | 58.74→59.48 | 70.07→70.83 | 75.23→75.72 | 57.28→57.69 | 78.60→79.45 | 61.67→61.78 | 43.97→44.07 | 92.07→92.43 |
| Ours | 78.87→79.80 | 55.36→56.73 | 53.89→56.27 | 73.09→73.21 | 54.99→55.38 | 83.42→83.48 | 46.51→46.69 | 30.28→30.36 | 90.31→90.65 |

Table 2. Quantitative comparison of post-hoc explanation methods on DenseNet-121. Format: Baseline→Ours.

| Method | CUB-200 | | | Oxford-IIIT Pet | | | Stanford Dogs | | |
|---|---|---|---|---|---|---|---|---|---|
| | Pixel Acc | mIoU | mAP | Pixel Acc | mIoU | mAP | Pixel Acc | mIoU | mAP |
| Saliency | 78.19→78.20 | 39.33→39.33 | 48.41→49.32 | 59.11→59.12 | 29.70→29.72 | 68.95→69.23 | 27.86→27.85 | 13.98→13.99 | 86.22→87.13 |
| GuidedBackprop | 78.18→78.20 | 39.20→39.25 | 64.81→65.19 | 59.04→59.07 | 29.58→29.63 | 64.18→64.79 | 27.76→27.77 | 13.90→13.90 | 89.15→90.04 |
| IntegratedGradients | 78.22→78.25 | 39.36→39.41 | 61.94→62.91 | 59.09→59.15 | 29.67→29.69 | 67.86→68.45 | 27.82→27.81 | 13.95→13.96 | 87.01→87.67 |
| GradCAM | 81.36→81.52 | 59.97→60.24 | 70.68→72.10 | 75.20→75.31 | 56.97→57.16 | 78.42→78.97 | 51.59→51.70 | 35.42→35.61 | 93.55→93.95 |
| GradCAM++ | 80.76→81.34 | 59.91→60.73 | 72.26→73.94 | 75.74→75.88 | 57.74→57.93 | 79.04→79.67 | 52.74→52.83 | 36.40→36.63 | 93.60→94.01 |
| ScoreCAM | 79.54→80.15 | 58.11→59.82 | 68.60→69.47 | 74.80→75.12 | 56.70→56.91 | 77.28→77.83 | 52.20→52.45 | 35.79→36.92 | 93.13→93.78 |
| Ours | 79.11→79.38 | 56.81→57.13 | 62.87→63.82 | 71.37→71.43 | 52.96→53.26 | 80.05→80.21 | 47.23→47.59 | 32.06→32.41 | 93.31→93.62 |

Table 3. Quantitative comparison of post-hoc explanation methods on ViT-B/32. Format: Baseline→Ours.

| Method | CUB-200 | | | Oxford-IIIT Pet | | | Stanford Dogs | | |
|---|---|---|---|---|---|---|---|---|---|
| | Pixel Acc | mIoU | mAP | Pixel Acc | mIoU | mAP | Pixel Acc | mIoU | mAP |
| Saliency | 78.31→78.32 | 39.79→39.80 | 57.85→58.56 | 59.17→59.18 | 29.84→29.86 | 65.42→65.97 | 27.92→27.93 | 14.05→14.06 | 85.77→85.93 |
| GuidedBackprop | 78.34→78.34 | 39.80→39.92 | 57.83→68.93 | 59.19→59.23 | 29.87→29.87 | 65.44→65.98 | 27.93→27.95 | 14.06→14.09 | 85.78→85.95 |
| IntegratedGradients | 78.28→78.28 | 39.61→39.62 | 64.86→65.24 | 59.12→59.13 | 29.71→29.75 | 61.05→62.19 | 27.85→27.87 | 13.98→14.05 | 84.23→85.04 |
| GradCAM | 65.40→65.87 | 36.32→36.41 | 34.79→35.35 | 51.66→52.58 | 28.01→28.69 | 44.57→44.60 | 40.59→40.96 | 22.48→22.52 | 73.06→73.68 |
| GradCAM++ | 64.54→65.79 | 35.85→36.02 | 35.41→35.92 | 51.08→52.53 | 27.62→28.40 | 43.90→44.86 | 38.76→39.07 | 21.11→21.42 | 71.79→71.93 |
| ScoreCAM | 81.33→81.42 | 54.35→55.13 | 66.24→66.83 | 64.16→64.60 | 39.69→39.97 | 67.14→67.29 | 33.40→33.92 | 18.99→18.70 | 85.56→85.63 |
| Ours | 83.95→84.23 | 63.64→64.29 | 74.87→75.92 | 71.08→71.35 | 52.06→52.38 | 79.15→79.72 | 46.36→46.58 | 31.44→31.67 | 93.02→93.25 |

To avoid outliers, we normalize using the 5% and 95% quantiles (computed via the differentiable approximation):

$$R_{\text{norm}} = \frac{R_{\text{gray}} - Q_{0.05}(R_{\text{gray}})}{Q_{0.95}(R_{\text{gray}}) - Q_{0.05}(R_{\text{gray}}) + \epsilon} \tag{4}$$

where $Q_p(\cdot)$ denotes the differentiable $p$-quantile and $\epsilon = 10^{-8}$ prevents division by zero.

#### 1.2.2. Step 2: Adaptive Soft Thresholding

We compute an adaptive threshold as the 80% quantile of the normalized map:

$$t_1 = Q_{0.8}(R_{\text{norm}}) \tag{5}$$

Instead of hard thresholding ($\mathbb{1}_{R_{\text{norm}}>t_1}$, which is non-differentiable), we use sigmoid-based soft thresholding:

$$R_{\text{high}} = \sigma\left(\beta(R_{\text{norm}} - t_1)\right) \tag{6}$$

where $\sigma(z) = 1/(1 + e^{-z})$ is the sigmoid function and $\beta = 10$ controls the steepness. As $\beta \to \infty$, this converges to the hard threshold.

#### 1.2.3. Step 3: Local Density Estimation

To suppress isolated noisy pixels, we compute local density via average pooling:

$$D = \text{AvgPool}_{31\times 31}(R_{\text{high}}) \tag{7}$$

with stride 1 and appropriate padding to maintain spatial dimensions. This operation is fully differentiable.

#### 1.2.4. Step 4: Final Mask Generation

The final mask is obtained by applying soft thresholding to the density map:

$$M = g(R) = \sigma\left(\beta(D - Q_{0.8}(D))\right) \tag{8}$$

## 2. Comparison with Post-hoc Explanation Methods Across All Architectures

In our experiments, we evaluate our approach on four representative architectures: ResNet-18, ResNet-50, DenseNet-121, and ViT-B/32. Due to space constraints in the main paper, we present detailed analysis on ResNet-50 as it represents the most widely-used baseline in computer vision

Table 4. Faithfulness evaluation on ResNet-18. Format: Baseline→Ours.

| Method | CUB-200 | | Pets | | Dogs | |
|---|---|---|---|---|---|---|
| | Insertion↑ | Deletion↓ | Insertion↑ | Deletion↓ | Insertion↑ | Deletion↓ |
| Saliency | 12.42→14.58 | 3.37→3.46 | 24.15→27.73 | 10.35→10.90 | 20.60→21.92 | 3.46→3.73 |
| GuidedBackprop | 17.33→19.12 | 2.75→2.72 | 33.74→35.93 | 7.34→7.98 | 26.55→28.70 | 3.48→3.77 |
| IntegratedGradients | 19.81→21.81 | 2.53→2.65 | 30.55→34.96 | 9.02→9.47 | 24.62→27.21 | 3.35→3.58 |
| GradCAM | 29.22→30.61 | 4.21→4.29 | 58.67→65.79 | 18.73→18.15 | 55.64→59.12 | 7.83→9.78 |
| GradCAM++ | 28.61→29.98 | 4.12→4.21 | 57.01→63.78 | 16.57→18.42 | 54.49→58.24 | 7.89→9.93 |
| ScoreCAM | 28.79→30.13 | 4.10→4.19 | 57.26→64.16 | 16.87→18.42 | 56.11→59.85 | 7.40→9.28 |
| Ours | 25.98→28.17 | 5.55→5.64 | 47.90→54.50 | 17.45→19.32 | 51.31→54.97 | 8.91→10.63 |

Table 5. Faithfulness evaluation on DenseNet-121. Format: Baseline→Ours.

| Method | CUB-200 | | Pets | | Dogs | |
|---|---|---|---|---|---|---|
| | Insertion↑ | Deletion↓ | Insertion↑ | Deletion↓ | Insertion↑ | Deletion↓ |
| Saliency | 16.83→26.57 | 3.83→4.37 | 28.42→32.53 | 12.12→15.01 | 32.99→43.61 | 5.21→11.60 |
| GuidedBackprop | 26.62→40.06 | 3.05→3.20 | 44.40→49.82 | 9.09→9.83 | 43.49→55.01 | 5.37→12.46 |
| IntegratedGradients | 26.51→39.60 | 3.24→3.45 | 39.73→44.93 | 12.48→13.36 | 37.59→52.01 | 5.25→10.15 |
| GradCAM | 46.10→63.36 | 5.95→7.16 | 62.79→69.65 | 16.41→17.66 | 63.05→79.75 | 8.54→12.80 |
| GradCAM++ | 45.40→62.02 | 6.20→7.49 | 61.84→68.65 | 16.61→17.87 | 62.54→78.87 | 8.73→13.19 |
| ScoreCAM | 45.30→61.99 | 6.72→8.40 | 61.37→67.68 | 17.95→20.24 | 62.21→76.37 | 9.93→15.44 |
| Ours | 39.74→53.53 | 9.44→11.28 | 53.82→58.92 | 20.74→22.45 | 58.49→73.79 | 9.70→17.13 |

Table 6. Faithfulness evaluation on ViT-B/32. Format: Baseline→Ours.

| Method | CUB-200 | | Pets | | Dogs | |
|---|---|---|---|---|---|---|
| | Insertion↑ | Deletion↓ | Insertion↑ | Deletion↓ | Insertion↑ | Deletion↓ |
| Saliency | 34.68→39.82 | 4.35→4.80 | 50.19→52.34 | 17.35→16.07 | 37.68→43.41 | 8.10→9.11 |
| GuidedBackprop | 34.73→40.03 | 4.39→4.97 | 50.23→52.47 | 17.33→16.35 | 37.73→43.47 | 8.12→9.15 |
| IntegratedGradients | 39.90→45.52 | 3.28→3.68 | 56.20→57.98 | 13.16→12.23 | 44.78→50.52 | 5.48→6.64 |
| GradCAM | 26.63→30.07 | 15.88→19.48 | 45.31→47.32 | 40.36→40.08 | 30.02→33.50 | 26.08→27.24 |
| GradCAM++ | 26.24→29.85 | 16.30→19.09 | 45.14→58.14 | 39.80→39.58 | 29.59→33.17 | 25.73→26.81 |
| ScoreCAM | 38.13→42.90 | 5.55→6.02 | 60.83→62.47 | 23.74→23.68 | 49.16→52.26 | 14.93→17.64 |
| Ours | 36.51→41.19 | 4.39→4.71 | 58.84→59.64 | 19.75→20.09 | 46.74→55.65 | 12.04→11.65 |

research. Here we provide complete quantitative results for the remaining three architectures. Tables 1, 2, and 3 show performance of six post-hoc explanation methods on ResNet-18, DenseNet-121, and ViT-B/32 respectively.

The results demonstrate that our training framework achieves consistent improvements across all architectures, datasets, and explanation methods. Similar to the ResNet-50 findings in the main paper, activation-based methods (GradCAM, GradCAM++, ScoreCAM) consistently show larger gains than gradient-based methods (Saliency, GuidedBackprop, IntegratedGradients) across all three architectures. For example, on CUB-200, ScoreCAM improves mIoU by +0.74 (ResNet-18), +1.71 (DenseNet-121), and +0.78 (ViT-B/32), while gradient-based methods typically show improvements below +0.10. Our proposed explanation method maintains strong performance across architectures, achieving mAP improvements of +2.38%/+0.95%/+1.05% on CUB-200 for ResNet-18/DenseNet-121/ViT-B/32 respectively. Notably, even on ViT-B/32 where GradCAM-based methods have lower baseline performance due to architectural mismatch with convolutional assumptions, our training framework still produces consistent improvements (e.g., GradCAM: +0.47% Pixel Acc, GradCAM++: +1.25% Pixel Acc on CUB-200), demonstrating the robustness of our information-theoretic approach across both convolutional

and transformer-based architectures.

## 3. Faithfulness Evaluation Across All Architectures

Tables 4, 5, and 6 present faithfulness evaluation results on ResNet-18, DenseNet-121, and ViT-B/32 respectively. The results demonstrate that the pattern observed in ResNet-50 generalizes consistently across all architectures: our training framework substantially improves Insertion scores while maintaining relatively stable Deletion performance.

Across all three architectures, we observe large Insertion improvements that indicate saliency maps better capture the features models actually use for classification. For instance, on CUB-200, GradCAM shows Insertion gains of +1.39 (ResNet-18), +17.26 (DenseNet-121), and +3.44 (ViT-B/32), while Deletion changes remain modest (+0.08, +1.21, +3.60 respectively). This asymmetric pattern—where Insertion gains substantially outweigh Deletion increases—holds across different explanation methods and datasets. Notably, DenseNet-121 exhibits particularly large improvements, with gradient-based methods (Saliency, GuidedBackprop, IntegratedGradients) achieving Insertion gains exceeding +10 points on CUB-200, likely due to DenseNet's dense connectivity structure being more amenable to our information-theoretic constraints. The consistency of these trends across diverse architectures validates that our approach fundamentally enhances model interpretability by aligning saliency maps with the model's true decision-making process.
